# Supplementary material for: MSF-Model: Queuing-Based Analysis and Prediction of Metastable Failures in Replicated Storage Systems
Source: arXiv:2309.16181 source file (2024-11-22)
Supplement: Supplementary file 1 [file appendix.tex]

\subsection{Queuing Model}

\subsubsection{Probability of Retry Calculation}
\label{appendix:prob_retry}
The probability of a retry is determined by the probability that a request's wait time exceeds the timeout duration. This probability is influenced by factors such as queue length, request processing rate, and timeout duration. The retry probability can be derived from the following:

\fontsize{8}{8}\selectfont
\begin{equation}
    P_{\text{retry}} = P(\text{Wait Time} > \tau)
    \label{eq:retry_probability}
\end{equation}
\normalsize

Here, $\tau$ denotes the timeout configured based on the system. The wait time is a function of the number of requests in the primary queue and the rate at which they are processed. We can rewrite this equation to account for these factors:

\fontsize{8}{8}\selectfont
\begin{equation}
    P_{\text{retry}} = P(N(\tau) \leq L)
\end{equation}
\normalsize

Here, $L$ represents the length of the primary queue, and $N(\tau)$ is the number of packets processed by the time $\tau$.
As the processing of each request follows an exponential distribution, this probability follows a Poisson process~\cite{kingman1992poisson}, which is calculated as follows:

\fontsize{8}{8}\selectfont
\begin{equation}
\begin{split}
     P_{\text{retry}} & = P(N(\tau) \leq L) \\
    & = P(N(\tau) = L) + P(N(\tau) = L-1) + \cdots + P\left( N(\tau) = 1 \right) \\
    & = \frac{(\mu \tau)^{L}}{L!}e^{-\mu \tau} +  \frac{(\mu \tau)^{(L-1)}}{(L-1)!}e^{-\mu \tau} + \cdots + e^{-\mu \tau}
\end{split}
\end{equation}
\normalsize

\subsubsection{Monte Carlo Analysis}
\label{appendix:monte_carlo}
Given our two-dimensional CTMC model, we can use the following steps to conduct a Monte Carlo analysis:

\begin{enumerate}[leftmargin=*]
    \item \textbf{Initialize}: Select an initial state $(i_0, j_0)$, where $i_0$ and $j_0$ are the initial numbers of requests in the orbit space and primary queue, respectively. Set a counter for each state to zero, and initialize the simulation time $t$ to zero.

    \item \textbf{Generate transition times}: For each possible transition from the current state $(i, j)$, draw a random number $r$ from the uniform distribution in the range $(0,1)$ and compute the corresponding exponential transition time $t_{i,j} = \frac{1}{- \text{rate}_{i,j}} \log(1 - r)$, where $\text{rate}_{i,j}$ is the transition rate for the specific transition as defined in the previous section. Keep track of the minimum transition time $t_{min}$ and the associated transition.

    \item \textbf{Update the state}: Perform the transition associated with the minimum transition time $t_{min}$, updating the state $(i, j)$ accordingly. Increment the counter for the new state and add the transition time $t_{min}$ to the simulation time $t$.

    \item \textbf{Check stopping criteria}: Evaluate the stopping criteria, which can be based on a predefined number of iterations, a fixed simulation time, or the convergence of the estimated probabilities. If the stopping criteria are not satisfied, return to step 2. Otherwise, proceed to the next step. Each of these stopping criteria is configurable based on the desired accuracy. In our experiments, we used fixed simulation time.

    \item \textbf{Compute stationary probabilities}: Divide the counter for each state by the total simulation time $t$ to obtain the estimated stationary probability for each state $(i, j)$. Normalize the probabilities so that they sum up to 1.
\end{enumerate}

By following these steps, the Monte Carlo simulation approximates the stationary probabilities of the CTMC, providing insights into the long-term behavior of the proposed queuing model. The estimated stationary probabilities can then be used to analyze and optimize the performance of the system, offering a practical approach to understanding the dynamics of our two-dimensional CTMC model.

\subsubsection{Generalizability of \ourModelName} 
\label{appendix:generalizability}
The primary focus of this part is to discuss the applicability and generalizability of \ourModel\ in various replication system configurations and to examine its capability in modeling metastable failures in complex systems. Figure~\ref{fig:model_generalization} represents different scenarios the model can capture. 

\begin{figure}[t]
    \centering
    \includegraphics[width=\linewidth]{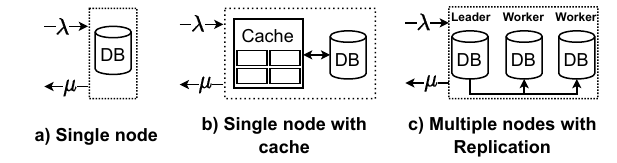}
    \caption{Different cases of a replicated storage system when a metastable failure can happen}
    \label{fig:model_generalization}
\end{figure}

\cat{Single Node without Replication} In this scenario, we treat the entire node as a server within our queuing model, with customers sending requests and retrials directly to the server. The model is applicable in this context, as the single node processes requests at a rate of $\mu$. Metastable failures may be triggered by an increase in incoming load (i.e., a higher $\lambda$) or a decline in system capacity (i.e., a lower $\mu$).

\cat{Standalone Node with Write-Through Cache}
The presence of a cache between the single node and customers does not affect the applicability of \ourModel. We can assume that the system processes requests at a dynamic rate of $\mu$, which may change upon cache failure. Consequently, metastable failures, in this case, may be triggered by alterations in system capacity. The entire system can be treated as a black box with a processing rate of $\mu$.

\cat{Multi-Node Replication System}
Replication across multiple nodes increases the overall processing time due to the time required for the replication process. This results in an increased processing rate for the entire system. \ourModel\ can still treat the entire system as if it is a single server. In the event of a trigger, such as a node crash-failure, the processing time and incoming load may change. The change in processing time occurs due to an altered replication process, while a node failure may cause a change in the incoming load as the affected node's customer requests are redirected to other nodes. Nevertheless, \ourModel\ remains applicable, as the important factors are the processing rate and incoming load.

% In more \textbf{Complex Systems}, \ourModel\ simplifies these systems by treating them as a single server with one queue, a method effective even for systems with multiple servers, parallel processing, or a network of queues. This model accurately represents systems where sequential request processing occurs or where multiple queues' effects are minimal. As a foundational element, \ourModel\ can be expanded to model more intricate systems, such as those represented by Directed Acyclic Graphs (DAG) involving interconnected subsystems. Each subsystem in such complex systems can be modeled using \ourModel\ as a basic unit, allowing the entire system to be represented through multiple instances of these units. This approach not only simplifies understanding of complex systems but also aids in analyzing various metastable failure scenarios. Additionally, the framework encompassing Modeling, Markov Chain construction, and Metastable Failure Analysis, based on queuing theory, offers a versatile and robust method for analyzing metastable failures in diverse systems.

\cat{Complex systems}
Certain real-world systems may be more complex, possibly employing multiple servers, parallel processing, or even a network of queues where tasks transition between different stages of processing. Some systems might also prioritize certain tasks over others or employ unique handling strategies. Despite these potential complexities, they can be accurately approximated using this single server and single queue model. Particularly, systems where requests are processed sequentially one after another or where the effects of multiple queues or servers are negligible can be well-represented by \ourModel.

\ourModel\ serves as a foundational block for modeling complex systems, such as those represented by Directed Acyclic Graphs (DAG) with multiple interconnected subsystems. Each subsystem within these complex structures can be effectively represented using our queuing framework, allowing the entire system to be modeled with multiple instances of these units. This modular approach enables \ourModel\ to adapt and expand, accommodating additional components as necessary to accurately reflect the specific characteristics and requirements of various complex systems.

In addition to the mentioned scenarios, the proposed framework for analyzing metastable failures---which incorporates Modeling, Markov Chain construction, and Metastable Failure Analysis---offers an efficient approach that can be readily applied to heterogeneous systems. This framework leverages the mathematical foundations of queuing theory to provide a robust analysis of this particular type of failure.
